# Supplementary material for: Self-consistent hybrid functional for condensed systems
Source: arXiv:1501.03184 source file (2015-01-13)
Supplement: Supplementary file 1 [file scHybrid-SM.pdf]

# Supplemental Material for:

# A self-consistent hybrid functional for condensed systems

Jonathan H Skone,[†] Marco Govoni,[‡] and Giulia Galli[*,‡]

*Department of Chemistry, University of California Davis, One Shields Ave., Davis, CA 95616, and Institute for Molecular Engineering, University of Chicago, 5801 South Ellis Avenue, Chicago, IL 60637*

E-mail: gagalli@uchicago.edu

The details of the basis sets used for each element are provided in Table S1. We either used Ahlrich's def2-TZVPP basis set as is (as in the case of H and O) or we modified the valence shell of the basis to avoid linear dependencies. In modifying the basis we removed any exponents smaller than 0.09 and then augmented and reoptimized the valence shell basis to maintain the original number of basis functions. In some cases we relaxed this constraint (Li, B, C, Mg, Ge, Mn, Co, and Ni) and the modified basis set for the solid is slightly smaller than the original def2 molecular basis set. The Co and Ni basis sets are the modified def2-TZVP of Bredow *et. al.*[1]

We compared the electronic dielectric constants and electronic energy gaps evaluated using the mod-def2-TZVPP Gaussian basis set and the CRYSTAL09 package[2] to results obtained with planewave pseudopotentials and the Qunatum-Espresso package[3] in Table S2. The *k*-point mesh used for each system (yielding converged values of the dielectric constant to within 0.05) is also

[*]To whom correspondence should be addressed
[†]Department of Chemistry, University of California Davis, One Shields Ave., Davis, CA 95616
[‡]Institute for Molecular Engineering, University of Chicago, 5801 South Ellis Avenue, Chicago, IL 60637

reported in Table S2. All ground state energies and energy gaps are converged to within 0.5 meV and 10 meV, respectively with this *k*-point mesh. For the CRYSTAL09 calculations, we used an energy tolerance for SCF convergence of $10^{-8}$ hartrees. The two-electron integral truncation tolerances were set in the following way: overlap threshold and penetration threshold for Coulomb integrals and overlap threshold for nonlocal exchange integrals were set at $10^{-8}$, and the two pseudo-overlap thresholds for the truncation of nonlocal exchange used were $10^{-8}$, and $10^{-16}$, respectively. The predefined extra large integration grid (XLGRID) was used for all systems–see the CRYSTAL09 manual for further details regarding the integration grid and the two-electron trunctation tolerances.

**Table S1:** Number of contracted basis functions (s/p/d/f) in our mod-TZVPP crystalline basis set, and Ahlrich's original def2-TZVPP molecular basis set,[4] for each element considered in the present study. Each entry in the Number of functions column corresponds to a function, where the number 1 indicates an uncontracted Gaussian and numbers larger than 1 indicate the function is contracted to one Gaussian function by the indicated number of primitive Gaussian functions. The Hf and W basis sets were optimized by other authors for use with the effective core potentials and are not included in this table (see references[5] and[6] for the optimized valence basis sets of Hf and W, respectively, used with the small core Hay-Wadt ECPs.[7]) The basis set information shown for Ne and Ar are for Ahlrich's def2-QZVPD molecular basis[8] and the corresponding modified crystalline basis. Though Ahlrich's def2 basis set contains higher angular momentum functions for some elements, we do not consider anything beyond f functions in the present work.

| | mod-def2-TZVPP crystalline | | Ahlrich's def2-TZVPP molecular | |
|---|---|---|---|---|
| Element | Number of functions (s/p/d/f) | Most diffuse s//p//d//f | Number of functions (s/p/d/f) | Most diffuse s//p//d//f |
| H | Unmodified | | 311/11/1/0 | 0.103//0.388//1.057//0.0 |
| Li | 62111/111/0/0 | 0.090//0.145//0.0//0.0 | 62111/111/1/0 | 0.029//0.060//0.132//0.0 |
| B | 6211/411/11/0 | 0.227//0.229//0.681//0.0 | 62111/411/11/1 | 0.061//0.065//0.199//0.490 |
| C | 6211/41/11/1 | 0.230//0.289//0.318//0.761 | 62111/411/11/1 | 0.095//0.101//0.318//0.761 |
| N | 621111/411/11/1 | 0.176//0.143//0.469//0.400 | 62111/411/11/1 | 0.136//0.143//0.469//1.093 |
| O | Unmodified | | 62111/411/11/1 | 0.185//0.175//0.645//1.428 |
| F | 62111/411/11/1 | 0.295//0.217//0.855/0.800 | 62111/411/11/1 | 0.240//0.217//0.855//1.917 |
| Ne | 82111111/6111/1111/11 | 0.095//0.169//0.347//1.524 | 821111111/61111/1111/11 | 0.106//0.047//0.198//1.524 |
| Na | 732111/511/11/0 | 0.100//0.101//0.330//0.0 | 73211/5111/111/0 | 0.019//0.091//0.100//0.0 |
| Mg | 73211/511/11/0 | 0.105//0.188//0.290//0.0 | 73211/5111/111/0 | 0.037//0.054//0.070//0.0 |
| Al | 732111/51111/111/11 | 0.201//0.152//0.180//0.451 | 73211/51111/111/1 | 0.060//0.058//0.110//0.244 |
| Si | 73211/51111/111/1 | 0.137//0.106//0.160//0.336 | 73211/51111/111/1 | 0.086//0.070//0.160//0.336 |
| P | 73211/51111/111/11 | 0.114//0.090//0.258//0.250 | 73211/51111/111/1 | 0.114//0.090//0.218//0.452 |
| S | 73211/51111/111/1 | 0.146//0.108//0.273//0.460 | 73211/51111/111/1 | 0.146//0.108//0.273//0.557 |
| Cl | 73211/51111/111/1 | 0.126//0.131//0.137//0.300 | 73211/51111/111/1 | 0.180//0.131//0.339//0.706 |
| Ar | (10)311111111/821111/11111/11 | 0.090//0.109//0.101//0.543 | (10)311111111/8211111/1111/11 | 0.065//0.030//0.101//0.543 |
| Ti | 842111/63111/4111/11 | 0.212//0.251//0.263//0.362 | 842111/63111/4111/11 | 0.033//0.054//0.054//0.254 |
| Mn | 842111/63111/411/11 | 0.101//0.205//0.228//0.726 | 842111/63111/4111/11 | 0.039//0.076//0.086//0.720 |
| Co | 84211/6311/411/1 | 0.136//0.702//0.292//1.903 | 842111/63111/4111/11 | 0.044//0.091//0.098//0.965 |
| Ni | 842111/6311/411/1 | 0.168//0.428//0.317//2.174 | 842111/63111/4111/11 | 0.047//0.099//0.106//1.087 |
| Zn | 842111/63111/4111/1 | 0.102//0.101//0.181//2.614 | 842111/63111/4111/11 | 0.051//0.048//0.124//1.433 |
| Ga | 842111/63111/5311/11 | 0.150//0.110//0.134//0.300 | 842111/63111/53111/1 | 0.072//0.063//0.114//0.310 |
| Ge | 84211/6311/5111/1 | 0.118//0.212//0.131//1.010 | 842111/63111/5111/1 | 0.094//0.086//0.132//0.362 |

**Table S2:** Comparison of the electronic dielectric constants ($\varepsilon_\infty$) and electronic energy gaps ($E_g$) evaluated with the all-electron mod-def2-TZVPP Gaussian type orbital (GTO) basis sets and with a plane-wave basis using pseudopotentials (PW pp). Calculations were carried out at the PBE level of theory. The GTO results were obtained with an all-electron basis set, with the exception of Hf and W, for which effective core potentials were used. In all PW pp calculations we used projector augmented wave type pseudopotentials with two exceptions, $WO_3$ and Ne, for which norm conserving pseudopotentials (Hartwigsen-Goedecker-Hutter type for Ne and Troullier-Martins type for Ne) were used. We used $k$-point meshes adequate to converge the values of the dielectric constants (see text). All local field effects were included in the evaluation of $\varepsilon_\infty$ (RPA + $f_{xc-l}$). All structures/polytypes for each system are the same as indicated in the main article, with ZnO being the only exception, where in this table we used the zinc-blende structure.

| System | N. atoms in cell | $k$-point mesh (N×N×N) | $\varepsilon_\infty$ GTO | $\varepsilon_\infty$ PW pp | $E_g$ (eV) GTO | $E_g$ (eV) PW pp |
|---|---|---|---|---|---|---|
| Ge | 2 | 20 | | | | |
| Si | 2 | 16 | 12.62 | 12.93 | 0.62 | 0.57 |
| AlP | 2 | 12 | 7.82 | 8.11 | 1.64 | 1.57 |
| SiC | 2 | 16 | 6.94 | 6.97 | 1.37 | 1.36 |
| $TiO_2$ | 6 | 10×10×8 | 7.91 | 7.82 | 1.81 | 1.90 |
| NiO | 4 | 12 | 16.98 | 16.87 | 0.97 | 0.95 |
| C | 2 | 16 | 5.83 | 5.84 | 4.15 | 4.14 |
| CoO | 4 | 12 | | | | |
| GaN | 2 | 14 | 5.78 | 6.00 | 1.88 | 1.67 |
| ZnS | 2 | 12 | 5.58 | 5.70 | 2.36 | 2.24 |
| MnO | 4 | 12 | 7.62 | 7.92 | 1.12 | 0.88 |
| $WO_3$ | 32 | 4 | 5.46 | 5.43 | 1.92 | 1.98 |
| BN | 2 | 12 | 4.59 | 4.60 | 4.49 | 4.47 |
| $HfO_2$ | 12 | 8 | 4.54 | | 4.32 | |
| AlN | 4 | 8 | 4.54 | 4.40 | 4.33 | 4.21 |
| ZnO (ZB) | 2 | 16 | 4.88 | 4.87 | 0.94 | 0.91 |
| $Al_2O_3$ | 10 | 4 | 3.27 | 3.23 | 6.31 | 6.31 |
| MgO | 2 | 8 | 3.12 | 3.11 | 4.80 | 4.77 |
| LiCl | 2 | 8 | 2.96 | 3.00 | 6.54 | 6.45 |
| NaCl | 2 | 8 | 2.49 | 2.52 | 5.18 | 5.23 |
| LiF | 2 | 8 | 1.97 | 2.06 | 9.21 | 9.19 |
| $H_2O$ | 12 | 3×3×2 | 1.80 | 1.85 | 5.57 | 5.56 |
| Ar | 1 | 8 | 1.74 | 1.74 | 8.78 | 8.70 |
| Ne | 1 | 8 | 1.28 | 1.29 | 11.65 | 11.57 |

## References


(1) Peintinger, M. F.; Oliveira, D. V.; Bredow, T. *Journal of computational chemistry* **2012**, *34*, 451–459.

(2) Dovesi, R.; Orlando, R.; Civalleri, B.; Roetti, C.; Saunders, V. R.; Zicovich-Wilson, C. M. *Zeitschrift für Kristallographie* **2005**, *220*, 571–573.

(3) Giannozzi, P. et al. *Journal of Physics: Condensed Matter* **2009**, *21*, 395502.

(4) Weigend, F.; Ahlrichs, R. *Physical Chemistry Chemical Physics* **2005**, *7*, 3297–3305.

(5) Muñoz Ramo, D.; Gavartin, J.; Shluger, A.; Bersuker, G. *Physical Review B* **2007**, *75*, 205336.

(6) Wang, F.; Di Valentin, C.; Pacchioni, G. *The Journal of Physical Chemistry C* **2011**, *115*, 8345–8353.

(7) Hay, P. J.; Wadt, W. R. *The Journal of chemical physics* **1985**, *82*, 299–310.

(8) Rappoport, D.; Furche, F. *The Journal of Chemical Physics* **2010**, *133*, 134105.
